# Supplementary material for: LEAD: Iterative Data Selection for Efficient LLM Instruction Tuning
Source: arXiv:2505.07437 source file (2025-05-12)
Supplement: Supplementary file 1 [file appendix.tex]

\section{Theoretical Guarantees}\label{sec:prooof1}
We present a theoretical framework for the analysis of our constraint single-objective optimization approach combining bandit algorithms with utility smoothing. The analysis consists of two main parts: first, deriving an approximation for loss changes during training, and second, determining the optimal smoothing coefficient that balances exploitation and exploration.

\subsection{Loss Changes in Gradient-Based Approximation}

\yuyu{Recap that we have introduced xxx in Section~\ref{secid}, [add details if necessary]. In this section, we try to ...[What]}.

\yuyu{[How]}
We begin by establishing the fundamental relationships between parameter updates and loss changes in gradient-based optimization.  
%Our hypothesis assumes that the current gradient is correlated with both the historical gradient from the same cluster and the gradient from the previous time step.

\qyl{
Recap that we have introduced approximation of uncertainty IU change in Section \ref{sec:details}. This approach allows us to efficiently estimate the approximate loss changes from the previous step ($\Delta L'(\theta_i, S_i)$) when model parameters are updated, without requiring additional computation, as established in \textbf{Theorem \ref{the:iuchange}}}

\qyl{In this section, we try to develop the theoretical foundation for approximating uncertainty changes. \textbf{Theorem \ref{proof:iu_change_approximation}} provides the formal derivation for these approximations, building upon the Loss Reduction-Gradient Relation established in \textbf{Lemma \ref{proof:loss_change}}. Our approach strategically leverages the correlation between current and historical gradient directions, with the precise assumptions formalized in \textbf{Hypothesis \ref{proof:hypothesis}}. This framework enables efficient estimation of uncertainty changes using only information available during the standard training process.
}

 \begin{hypothesis}[Gradient Direction Correlation]
 \label{proof:hypothesis1}
 Let $C_k$ denote the cluster selected at step $t$, and $t_k$ be the most recent step when cluster $C_k$ was previously selected.
 The gradient direction at the current step $t$ is correlated with both the historical gradient direction of the selected cluster and the previous step's gradient, represented as:
\begin{equation} \small
    \nabla L'(S_t,\theta_{t-1}) \equiv  \beta \cdot \nabla L(S_{t_k}, \theta_{t_k-1}) + (1-\beta) \cdot \nabla L(S_{t-1},\\theta_{t-2})
\end{equation}
where $\beta \in [0,1]$ is a weighting coefficient measuring the relative importance of cluster-specific historical information versus recent optimization direction.
\end{hypothesis}

\begin{theorem}[IU Change Approximation]
\label{proof:iu_change_approximation1}
For any sample set $S_t$, the average uncertainty change $\Delta L'(\theta_t, S_t)$ when model parameters update from $\theta_{t-1}$ to $\theta_t$ can be approximated as:
\begin{align} \small
    \delta_t &\equiv\Delta L'(\theta_t, S_t) \\
    &= -\eta\Big[\beta^2\delta_{t_k} + (1-\beta)^2\delta_{t-1}  + 2\beta(1-\beta)\sqrt{\delta_{t_k}\delta_{t-1}}\cos\phi\Big]
\end{align}
where $\phi$ is the angle between parameter update directions $\Delta\theta_{t_k}$ and $\Delta\theta_{t-1}$, with $\cos\phi = \frac{\Delta\theta_{t_k}^{\top}\Delta\theta_{t-1}}{\|\Delta\theta_{t_k}\|\|\Delta\theta_{t-1}\|}$.

Furthermore, the optimal weighting coefficient $\beta^*$ that minimizes the approximation error
\begin{equation} \small
J(\beta) = \|\nabla L_t - (\beta \nabla L_{t_k} + (1-\beta)\nabla L_{t-1})\|^2
\end{equation}
is given by
\begin{equation} \small
\beta^* = \frac{\delta_{t-1} - \sqrt{\delta_{t_k}\delta_{t-1}}\cos\phi}{\delta_{t_k} + \delta_{t-1} - 2\sqrt{\delta_{t_k}\delta_{t-1}}\cos\phi}
\end{equation}
% $\delta_t = -\eta\|\nabla L_t\|^2$ represents the loss reduction.
\end{theorem}

\begin{proof}
We begin by expressing the error in approximating the current gradient by a convex combination of two previous gradients:
\begin{equation} \small
J(\beta) = \left\|\nabla L_t - \left[ \beta\, \nabla L_{t_k} + (1-\beta)\, \nabla L_{t-1} \right] \right\|^2.
\end{equation}
Using the standard gradient descent update rule
\[
\Delta\theta_t = -\eta\, \nabla L_t,
\]
we can rewrite the gradients in terms of parameter updates:
\begin{equation} \small
\nabla L_t = -\frac{\Delta\theta_t}{\eta}, \quad
\nabla L_{t_k} = -\frac{\Delta\theta_{t_k}}{\eta}, \quad 
\nabla L_{t-1} = -\frac{\Delta\theta_{t-1}}{\eta}.
\end{equation}
Substituting these relationships into the error function yields
\begin{align} \small
J(\beta) &= \left\| -\frac{\Delta\theta_t}{\eta} - \left[-\frac{1}{\eta}\Bigl(\beta\, \Delta\theta_{t_k} + (1-\beta)\, \Delta\theta_{t-1}\Bigr) \right] \right\|^2 \notag\\[1mm]
&= \frac{1}{\eta^2}\left\|\Delta\theta_t - \Bigl(\beta\, \Delta\theta_{t_k} + (1-\beta)\, \Delta\theta_{t-1}\Bigr) \right\|^2.
\end{align}
For simplicity, we define 
\[
\mathbf{E}(\beta) = \Delta\theta_t - \Bigl(\beta\, \Delta\theta_{t_k} + (1-\beta)\, \Delta\theta_{t-1}\Bigr).
\]
Since the constant factor $1/\eta^2$ does not affect the minimizer, we focus on minimizing 
\begin{equation} \small
\tilde{J}(\beta) = \|\mathbf{E}(\beta)\|^2.
\end{equation}
According to Lemma \ref{proof:loss_change}, we have: 
\begin{equation} \small
\|\nabla L(S_{t_k}, \theta_{t_k-1})\| \approx \sqrt{\frac{-\delta_{t_k}}{\eta}},
\end{equation}
with an analogous relation for $\nabla L_{t-1}$. This allows us to write
\[
\|\Delta\theta_{t_k}\|^2 \approx -\eta\, \delta_{t_k}, \qquad \|\Delta\theta_{t-1}\|^2 \approx -\eta\, \delta_{t-1}.
\]
Define the cosine of the angle between parameter updates as:
\[
\cos\phi = \frac{\Delta\theta_{t_k}^{\top}\Delta\theta_{t-1}}{\|\Delta\theta_{t_k}\|\|\Delta\theta_{t-1}\|}.
\]
Without loss of generality, we assume that the contribution of $\Delta\theta_t$ can be related to those of $\Delta\theta_{t_k}$ and $\Delta\theta_{t-1}$. Under this assumption, differentiating $\tilde{J}(\beta)$ with respect to $\beta$ and setting the derivative to zero:
\begin{equation} \small
\frac{d\tilde{J}}{d\beta}=0 \quad \Longrightarrow \quad \beta^* = \frac{\delta_{t-1} - \sqrt{\delta_{t_k}\delta_{t-1}}\, \cos\phi}{\delta_{t_k} + \delta_{t-1} - 2\sqrt{\delta_{t_k}\delta_{t-1}}\, \cos\phi}.
\end{equation}
Using the optimal $\beta^*$, the loss change at step $t$ is approximated by:
\begin{align} \small
\delta_t &= \Delta L'(\theta_t, S_t) \\
&= -\eta\Bigl[(\beta^*)^2\, \delta_{t_k} + (1-\beta^*)^2\, \delta_{t-1} + 2\,\beta^*(1-\beta^*)\,\sqrt{\delta_{t_k}\delta_{t-1}}\,\cos\phi\Bigr].
\end{align}
\end{proof}

\begin{comment}
    \begin{theorem}[IU Change Approximation]
\label{proof:iu change approximation1}
For any sample set $S_i$, the average uncertainty change $\Delta L'(\boldsymbol{\theta}_i, S_i)$ when model parameters update from $\boldsymbol{\theta}_{i-1}$ to $\boldsymbol{\theta}_i$ can be approximated as:
\begin{align}
    \delta_t &\equiv\Delta L'(\boldsymbol{\theta}_i, S_i) \\
    &= -\eta\Big[\beta^2\delta_{i_k} + (1-\beta)^2\delta_{i-1}  + 2\beta(1-\beta)\sqrt{\delta_{i_k}\delta_{i-1}}\cos\phi\Big]
\end{align}
where $\phi$ is the angle between parameter update directions $\Delta\theta_{i_k}$ and $\Delta\theta_{i-1}$, with $\cos\phi = \frac{\Delta\theta_{i_k}^{\top}\Delta\theta_{i-1}}{\|\Delta\theta_{i_k}\|\|\Delta\theta_{i-1}\|}$.
\end{comment}

\begin{lemma}[Loss Reduction-Gradient Relation]
\label{proof:loss_change1}
For any sample set $S_t$, the average loss change when model parameters update from $\theta_{t-1}$ to $\theta_t$ can be approximated as:
\begin{equation}\small
 \Delta L(\theta_t, S_t) = \frac{1}{|S_t|}\sum_{x\in S_t}(L(\theta_t, x) - L(\theta_{t-1}, x)) \approx -\eta_t \|\nabla L(\theta_{t-1}, S_t)\|^2
\end{equation}
\end{lemma}

\begin{proof}
Assume at round $t$, model parameters are updated via gradient descent:
\begin{equation} \small
    \theta_t = \theta_{t-1} - \eta_t\nabla L(S_t, \theta_{t-1})
\end{equation}

where $\nabla L(S_t, \theta_{t-1}) = \frac{1}{|S_t|}\sum_{x\in S_t}\nabla L(x, \theta_{t-1})$ is the average gradient of subset $S_t$.

For each sample $x \in S_t$, the loss function $L(\theta, x)$ is expanded using first-order Taylor expansion at $\theta_{t-1}$:
\begin{equation} \small
    L(\theta_t, x) \approx L(\theta_{t-1}, x) + \nabla L(\theta_{t-1}, x)^{\top}(\theta_t - \theta_{t-1})
\end{equation}

Substituting the parameter update formula:
\begin{equation} \small
    L(\theta_t, x) - L(\theta_{t-1}, x) \approx -\eta_t\nabla L(\theta_{t-1}, x)^{\top}\nabla L(\theta_{t-1}, S_t)
\end{equation}

Averaging over all samples in $S_t$:
\begin{align} \small
 \delta_t=\Delta L(\theta_t, S_t) &= \frac{1}{|S_t|}\sum_{x\in S_t}(L(\theta_t, x) - L(\theta_{t-1}, x))\\
    &\approx -\eta_t\frac{1}{|S_t|}\sum_{x\in S_t}\nabla L(\theta_{t-1}, x)^{\top}\nabla L(\theta_{t-1}, S_t)\\
    &= -\eta_t\|\nabla L(\theta_{t-1}, S_t)\|^2
\end{align}
\end{proof}

\subsection{Optimal Smoothing Coefficient}

\qyl{Recap that we introduced a novel smoothed utility function in Section \ref{sec:Instance-Level Dynamic Uncertainty}, which effectively integrates both current and historical information.  The precise mathematical formulation is presented in Definition \ref{def:idu}.}

\qyl{In this section, we establish the theoretical foundation for optimizing this function.  First, Lemma \ref{lemma:Utility Change Decomposition} provides a precise mathematical presentation for smoothed utility function changes, which shows the relationship between $\Delta IDU$ and the size of batch $S_t$. 
Then, Lemma \ref{proof:expected sample size}  derives a closed-form expression for the expected sample size in the t-th training round.
Building upon these results, Theorem \ref{proof:optimal smoothing coefficient} determines the optimal smoothing coefficient that maximizes cumulative utility gain while respecting budget constraints.
 Finally, Corollary \ref{proof:min training steps} establishes the minimum number of training rounds required to satisfy these constraints.}

\begin{lemma}[Batch Utility Change Decomposition]
\label{lemma:Utility Change Decomposition1}
The utility change for batch $S_t$ under smoothed utility function can be expressed as:
\begin{equation} \small
\Delta IDU_t = 
\begin{cases} 
-(1-b)\eta_t |S_t| \Psi_t + b |S_t| \delta_{t-1}(1 - b^{t-1}), & t \leq 5 \\
-(1-b)\eta_t |S_t| \Psi_t, & t > 5 
\end{cases}
\end{equation}
where $\Psi_t$ denotes the gradient alignment term:
\begin{equation} \small
\Psi_t = \beta_t^2 \delta_{t_k} + (1-\beta_t)^2 \delta_{t-1} + 2\beta_t(1-\beta_t)\sqrt{\delta_{t_k}\delta_{t-1}}\cos\phi_t
\end{equation}
\end{lemma}

\begin{proof}
We begin by expressing the per-sample utility change. For any sample $x \in S_t$, the utility change under our smoothed utility function is given by:
\begin{align} \small
\Delta IDU_t(x) &=IDU(\theta_t, x) -IDU(\theta_{t-1}, x) \\
&= (1-b)L(\theta_t, x) + bL'(\theta_{t-1}, x) -IDU(\theta_{t-1}, x) \\
&= (1-b)[L(\theta_t, x) - L(\theta_{t-1}, x)] \\& + (1-b)[L(\theta_{t-1}, x) -IDU(\theta_{t-1}, x)]
\end{align}

The first term $L(\theta_t, x) - L(\theta_{t-1}, x) = \Delta L(\theta_t, x)$ represents the immediate loss change. For the second term, by recursive expansion of $L'(\theta_{t-1}, x)$:
\begin{align} \small
IDU(\theta_{t-1}, x) &= (1-b)L(\theta_{t-1}, x) + b\dot IDU(\theta_{t-2}, x) \\
&= (1-b)\sum_{k=0}^{t-2} b^k L(\theta_{t-1-k}, x) + b^{t-1}IDU(\theta_0, x)
\end{align}

Therefore, 
\begin{align}\small
&(1-b)[L(\theta_{t-1}, x) -IDU(\theta_{t-1}, x)] \nonumber \\
&= (1-b)L(\theta_{t-1}, x) - (1-b)^2\sum_{k=0}^{t-2} b^k L(\theta_{t-1-k}, x) \\& -  (1-b)b^{t-1}IDU(\theta_0, x) \\
&= b(1-b)\sum_{k=0}^{t-3} b^{k} L(\theta_{t-2-k}, x)  \\& + (1-b)b^{t-1}IDU(\theta_0, x) 
\end{align}

Combining the terms, we obtain:
\begin{align} \small
\Delta IDU_t(x) &= (1-b)\Delta L(\theta_t, x) \\
&+ b(1-b)\sum_{k=0}^{t-3} b^{k} L(\theta_{t-2-k}, x) + (1-b)b^{t-1}IDU(\theta_0, x)
\end{align}

By the gradient alignment hypothesis, the immediate loss change can be expressed as:
\begin{align}\small 
\delta_t &\approx -\eta_t\Big[\beta_t^2 \delta_{t_k} + (1-\beta_t)^2 \delta_{t-1} 
+ 2\beta_t(1-\beta_t)\sqrt{\delta_{t_k}\delta_{t-1}}\cos\phi_t\Big] \\
& = -\eta_t\Psi_t
\end{align}

For the historical terms, we can approximate:
\begin{align}\small
\sum_{k=0}^{t-3} b^{k} [L(\theta_{t-2-k}, x) - L(\theta_{t-3-k}, x)] &\approx \delta_{t-1}\sum_{k=0}^{t-3} b^{k} \\
&= \delta_{t-1}\frac{1 - b^{t-2}}{1 - b}
\end{align}

Where $\delta_{t-1}$ represents the average loss change in recent iterations.

For the term involving $IDU(\theta_0, x)$, we can treat it as a constant initial condition $C_0$.

Aggregating over all samples in batch $S_t$, we obtain:
\begin{align} \small
\Delta IDU_t &= \sum_{x \in S_t} \Delta IDU_t(x) \\
&= (1-b)\sum_{x \in S_t}\Delta L(\theta_t, x) + b(1-b)\sum_{x \in S_t}\sum_{k=0}^{t-3} b^{k} L(\theta_{t-2-k}, x) \nonumber \\
&\quad + (1-b)b^{t-1}\sum_{x \in S_t}IDU(\theta_0, x) \\
&= -(1-b)\eta_t |S_t|\Psi_t + b|S_t|\delta_{t-1}(1-b^{t-2}) 
\\ \quad &+ (1-b)b^{t-1}|S_t|C_0
\end{align}

For practical purposes, we can absorb this term into our approximation and express:
\begin{align} \small
\Delta IDU_t \approx -(1-b)\eta_t |S_t|\Psi_t + b|S_t|\delta_{t-1}(1-b^{t-1})
\end{align}

This expression is valid for all $t$. However, for $t > 5$ and typical values of $b < 1$, the term $b^{t-1}$ becomes negligibly small (e.g., if $b = 0.5$, then $b^5 = 0.03125$), and we can simplify to:

\begin{align} \small
\Delta IDU_t \approx -(1-b)\eta_t |S_t|\Psi_t \quad \text{for } t > 5
\end{align}
\end{proof}

\begin{lemma}[Expected Sample Size Under MAB mechanism]
\label{proof:expected sample size1}
In the MAB framework using EXP3.S for cluster selection with smoothed utility, the expected sample size per round $\mathbb{E}[n_t]$ satisfies:
\begin{equation} \small
%\mathbb{E}[n_t] = \alpha \cdot (1-b) \cdot \frac{\sum_{i=1}^K |C_i|^2}{\sum_{i=1}^K |C_i|} \cdot \left(1 + \mathcal{O}(\gamma)\right)
\mathbb{E}[n_t] = \alpha \cdot (1-b) \cdot \overline{|C|} \cdot (1 + \text{CV}^2) \cdot \left(1 + \mathcal{O}(\gamma)\right)
\end{equation}
where $\alpha$ is the base sampling rate, $b$ is the smoothing coefficient, $|C_i|$ is the size of cluster $i$, and $\gamma$ is the exploration rate in  EXP3.S algorithm \ref{MAB_algorithm}.
\end{lemma}

\begin{proof}
We analyze cluster selection probabilities in the EXP3.S algorithm when used with our smoothed utility rewards. The reward signal for selecting cluster $i$ at time $t$ is:
\begin{equation} \small
R_i^{(t)} = \Delta IDU_t \propto (1-b)|C_i|
\end{equation}

This relationship follows directly from Theorem 1 (Batch Utility Change Decomposition) for $t > 5$, where $\Delta IDU_t = -(1-b)\eta_t |S_t| \Psi_t$. Since $|S_t|$ is proportional to cluster size $|C_i|$ when cluster $i$ is selected, and assuming $\Psi_t$ and $\eta_t$ are approximately constant across clusters, we derive $R_i^{(t)} \propto (1-b)|C_i|$ after normalizing by the negative sign (as MAB maximizes rewards).

In the EXP3.S algorithm, the cluster selection probability is given by:
\begin{equation} \small
p_i^{(t)} = (1-\gamma)\frac{w_i^{(t)}}{\sum_{j=1}^K w_j^{(t)}} + \frac{\gamma}{K}
\end{equation}

The weights evolve according to:
\begin{equation} \small
w_i^{(t+1)} = w_i^{(t)} \exp\left(\frac{\gamma}{K}\frac{R_i^{(t)}}{p_i^{(t)}}\right) + \frac{\epsilon}{K}\sum_{j=1}^K w_j^{(t)}
\end{equation}

As the algorithm converges to steady state, the weights stabilize such that:
\begin{equation} \small
\frac{w_i^{(t)}}{\sum_{j=1}^K w_j^{(t)}} \propto \exp\left(\sum_{\tau=1}^{t-1}\frac{\gamma}{K}\frac{R_i^{(\tau)}}{p_i^{(\tau)}}\right)
\end{equation}

In the fully converged regime, assuming small $\gamma$ and $\epsilon$, and sufficiently heterogeneous cluster sizes, we can derive a fixed-point equation. At this fixed point, the ratio $\frac{R_i^{(t)}}{p_i^{(t)}}$ becomes approximately constant across arms, leading to:
\begin{equation} \small
p_i^{(t)} \approx \frac{(1-\gamma)(1-b)|C_i|}{\sum_{j=1}^K (1-b)|C_j|} + \frac{\gamma}{K} = \frac{(1-\gamma)(1-b)|C_i|}{\sum_{j=1}^K |C_j|} + \frac{\gamma}{K}
\end{equation}

For small $\gamma$, the dominant term is:
\begin{equation} \small
p_i^{(t)} \approx \frac{(1-b)|C_i|}{\sum_{j=1}^K |C_j|} + \mathcal{O}(\gamma)
\end{equation}

The expected sample size in round $t$ is:
\begin{align} \small
\mathbb{E}[n_t] &= \alpha \sum_{i=1}^K p_i^{(t)} |C_i| \\
&= \alpha \sum_{i=1}^K \left(\frac{(1-b)|C_i|}{\sum_{j=1}^K |C_j|} + \mathcal{O}(\gamma)\right) |C_i| \\
&= \alpha (1-b) \frac{\sum_{i=1}^K |C_i|^2}{\sum_{j=1}^K |C_j|} + \alpha \cdot \mathcal{O}(\gamma) \sum_{i=1}^K |C_i| \\
\end{align}

Since $\sum_{i=1}^K |C_i| = N$ (total dataset size), we can express this as:
\begin{equation} \small
\mathbb{E}[n_t] = \alpha \cdot (1-b) \cdot \frac{\sum_{i=1}^K |C_i|^2}{\sum_{i=1}^K |C_i|} \cdot \left(1 + \mathcal{O}(\gamma)\right)
\end{equation}

Let $\overline{|C|} = \frac{1}{K}\sum_{i=1}^K |C_i|$ be the average cluster size. Using the relation between variance and second moment:
\begin{equation} \small
\frac{1}{K}\sum_{i=1}^K |C_i|^2 = \text{Var}(|C_i|) + \overline{|C|}^2 = \overline{|C|}^2 \cdot \text{CV}^2 + \overline{|C|}^2 = \overline{|C|}^2 (1 + \text{CV}^2)
\end{equation}

Therefore:
\begin{align} \small
\frac{\sum_{i=1}^K |C_i|^2}{\sum_{i=1}^K |C_i|} &= \frac{K \cdot \overline{|C|}^2 (1 + \text{CV}^2)}{K \cdot \overline{|C|}} \\
&= \overline{|C|} \cdot (1 + \text{CV}^2)
\end{align}

Substituting into our expected sample size formula:
\begin{equation} \small
\mathbb{E}[n_t] = \alpha \cdot (1-b) \cdot \overline{|C|} \cdot (1 + \text{CV}^2) \cdot \left(1 + \mathcal{O}(\gamma)\right)
\end{equation}

\end{proof}

\begin{comment}
    \begin{corollary}[Effect of Cluster Size Heterogeneity]
The expected sample size can be expressed in terms of the coefficient of variation (CV) of cluster sizes:
\begin{equation}
\mathbb{E}[n_t] = \alpha \cdot (1-b) \cdot \overline{|C|} \cdot (1 + \text{CV}^2) \cdot \left(1 + \mathcal{O}(\gamma)\right)
\end{equation}
where $\overline{|C|} = \frac{1}{K}\sum_{i=1}^K |C_i|$ is the average cluster size and $\text{CV}^2 = \frac{1}{K}\sum_{i=1}^K \frac{(|C_i| - \overline{|C|})^2}{\overline{|C|}^2}$ is the squared coefficient of variation.
\end{corollary}

\begin{proof}
Let $\overline{|C|} = \frac{1}{K}\sum_{i=1}^K |C_i|$ be the average cluster size. Using the relation between variance and second moment:
\begin{equation}
\frac{1}{K}\sum_{i=1}^K |C_i|^2 = \text{Var}(|C_i|) + \overline{|C|}^2 = \overline{|C|}^2 \cdot \text{CV}^2 + \overline{|C|}^2 = \overline{|C|}^2 (1 + \text{CV}^2)
\end{equation}

Therefore:
\begin{align}
\frac{\sum_{i=1}^K |C_i|^2}{\sum_{i=1}^K |C_i|} &= \frac{K \cdot \overline{|C|}^2 (1 + \text{CV}^2)}{K \cdot \overline{|C|}} \\
&= \overline{|C|} \cdot (1 + \text{CV}^2)
\end{align}

Substituting into our expected sample size formula:
\begin{equation}
\mathbb{E}[n_t] = \alpha \cdot (1-b) \cdot \overline{|C|} \cdot (1 + \text{CV}^2) \cdot \left(1 + \mathcal{O}(\gamma)\right)
\end{equation}

This shows that greater cluster size heterogeneity (higher CV) leads to increased expected sample size, while higher smoothing coefficient $b$ reduces the expected sample size.
\end{proof}
\end{comment}

\begin{theorem}[Optimal Smoothing Coefficient]
\label{proof:optimal smoothing coefficient1}
The optimal smoothing coefficient $b^*$ that maximizes the cumulative utility gain under the budget constraint is:
\begin{equation} \small
b^* = 1 - \frac{B}{n_0 T \cdot (1 + \text{CV}^2)}
\end{equation}
where $n_0 = \alpha \cdot \overline{|C|}$ is the expected batch size without smoothing and heterogeneity effects, $B$ is the total budget, $T$ is the number of training steps, and $\text{CV}^2$ quantifies cluster size variability.
\end{theorem}

\begin{proof}
The utility-based reward for chosen cluster $i_t$ in the steady state ($t > 5$) is:
\begin{equation} \small
R^{(t)} = \Delta IDU_t = -(1-b)\eta_t|S_t|\Psi_t
\end{equation}

Let us denote $\mathbb{E}[|S_t|\Psi_t] = \delta_t \cdot \mathbb{E}[n_t]$, where $\delta_t$ represents the average per-sample utility contribution and $\mathbb{E}[n_t]$ is the expected sample size. From our analysis of the MAB framework:
\begin{equation} \small
\mathbb{E}[n_t] = \alpha \cdot (1-b) \cdot \frac{\sum_{i=1}^K |C_i|^2}{\sum_{i=1}^K |C_i|} \cdot \left(1 + \mathcal{O}(\gamma)\right)
\end{equation}

For small $\gamma$ and using the relationship between the sum of squared cluster sizes and the coefficient of variation:
\begin{equation} \small
\mathbb{E}[n_t] \approx \alpha \cdot (1-b) \cdot \overline{|C|} \cdot (1 + \text{CV}^2) = n_0 \cdot (1-b) \cdot (1 + \text{CV}^2)
\end{equation}
where $n_0 = \alpha \cdot \overline{|C|}$ represents the expected sample size without smoothing and heterogeneity effects.

The objective function becomes:
\begin{align} \small
\sum_{t=1}^T \mathbb{E}[\Delta IDU_t] &= -\sum_{t=1}^T (1-b)\eta_t \cdot \mathbb{E}[|S_t|\Psi_t] \\
&= -\sum_{t=1}^T (1-b)\eta_t \cdot \delta_t \cdot \mathbb{E}[n_t] \\
&= -\sum_{t=1}^T (1-b)\eta_t \cdot \delta_t \cdot n_0 \cdot (1-b) \cdot (1 + \text{CV}^2) \\
&= -n_0 \cdot (1-b)^2 \cdot (1 + \text{CV}^2) \cdot \sum_{t=1}^T \eta_t \delta_t
\end{align}

Let $\bar{\eta} \delta = \frac{1}{T}\sum_{t=1}^T \eta_t \delta_t$ be the average product of learning rate and utility contribution. The objective simplifies to:
\begin{equation} \small
\sum_{t=1}^T \mathbb{E}[\Delta IDU_t] = -n_0 \cdot T \cdot \bar{\eta} \delta \cdot (1-b)^2 \cdot (1 + \text{CV}^2)
\end{equation}

The budget constraint becomes:
\begin{align} \small
\sum_{t=1}^T \mathbb{E}[n_t] &= \sum_{t=1}^T n_0 \cdot (1-b) \cdot (1 + \text{CV}^2) \\
&= n_0 \cdot T \cdot (1-b) \cdot (1 + \text{CV}^2) \leq B
\end{align}

We formulate the Lagrangian:
\begin{equation} \small
\mathcal{L}(b,\lambda) = -n_0 \cdot T \cdot \bar{\eta} \delta \cdot (1-b)^2 \cdot (1 + \text{CV}^2) + \lambda(n_0 \cdot T \cdot (1-b) \cdot (1 + \text{CV}^2) - B)
\end{equation}

Taking the partial derivative with respect to $b$ and setting to zero:
\begin{align} \small
\frac{\partial \mathcal{L}}{\partial b} &= 2n_0 \cdot T \cdot \bar{\eta} \delta \cdot (1-b) \cdot (1 + \text{CV}^2) - \lambda \cdot n_0 \cdot T \cdot (1 + \text{CV}^2) = 0 \\
& \Rightarrow 2\bar{\eta} \delta \cdot (1-b) \\
&= \lambda
\end{align}

The complementary slackness condition states $\lambda(n_0 \cdot T \cdot (1-b) \cdot (1 + \text{CV}^2) - B) = 0$. Since $\lambda \neq 0$ (as verified by the optimality condition), the budget constraint must be tight:
\begin{equation} \small
n_0 \cdot T \cdot (1-b) \cdot (1 + \text{CV}^2) = B
\end{equation}

Solving for $b$:
\begin{equation} \small
b^* = 1 - \frac{B}{n_0 \cdot T \cdot (1 + \text{CV}^2)}
\end{equation}

For this solution to be valid, we require $0 \leq b^* < 1$, which implies:
\begin{equation} \small
T > \frac{B}{n_0 \cdot (1 + \text{CV}^2)}
\end{equation}

This provides the minimum number of training steps needed to satisfy our budget constraint with a valid smoothing coefficient.
\end{proof}

\begin{corollary}[Minimum Training Steps]
\label{proof:min training steps1}
The minimum number of training steps required to complete training under budget constraint $B$ is:
\begin{equation} \small
T_{\min} = \left\lceil\frac{B}{n_0 \cdot (1 + \text{CV}^2)}\right\rceil
\end{equation}
where $\lceil \cdot \rceil$ denotes the ceiling function.
\end{corollary}

\begin{proof}
From the constraint $b^* < 1$, we derive:
\begin{align} \small
1 - \frac{B}{n_0 \cdot T \cdot (1 + \text{CV}^2)} &< 1 \\
\Rightarrow \frac{B}{n_0 \cdot T \cdot (1 + \text{CV}^2)} &> 0 \\
\end{align}

Since all terms in the denominator are positive, this inequality is always satisfied. From the constraint $b^* \geq 0$, we derive:
\begin{align} \small
1 - \frac{B}{n_0 \cdot T \cdot (1 + \text{CV}^2)} &\geq 0 \\
\Rightarrow \frac{B}{n_0 \cdot T \cdot (1 + \text{CV}^2)} &\leq 1 \\
\Rightarrow T &\geq \frac{B}{n_0 \cdot (1 + \text{CV}^2)}
\end{align}

Since $T$ must be an integer, we take the ceiling:
\begin{equation} \small
T_{\min} = \left\lceil\frac{B}{n_0 \cdot (1 + \text{CV}^2)}\right\rceil + 1
\end{equation}

This represents the minimum number of training steps required to satisfy the budget constraint with a non-negative smoothing coefficient.
\end{proof}

\subsection{Example: Budget-Constrained Optimization}

To illustrate our approach, we analyze a dataset with 7 clusters $\{|C_i|\} = \{62828, 61844, 71712, 69728, 93923, 107415, 52574\}$ under a budget constraint $B = 15,000$ and sampling rate $\alpha = 0.015$.

With average cluster size $\overline{|C|} \approx 74,289$ and cluster size variation $\text{CV}^2 \approx 0.0586$, we calculate $n_0 = \alpha \cdot \overline{|C|} \approx 1,114$. Applying our theoretical results:

\begin{align} \small
T_{\min} &= \left\lceil\frac{B}{n_0 \cdot (1 + \text{CV}^2)}\right\rceil + 1 = 14\\
b^* &= 1 - \frac{B}{n_0 \cdot T_{\min} \cdot (1 + \text{CV}^2)} \approx 0.092
\end{align}

This indicates 14 training steps with smoothing coefficient 0.092 optimally balances utility maximization and budget constraints for this heterogeneous cluster distribution.
